# Supplementary material for: Folding Polyiamonds into Octahedra
Source: arXiv:2207.13989 source file (2022-07-28)
Supplement: Supplementary file 1 [file 07-Appendix.tex]

\setcounter{section}{1}
\section{Details of \cref{sec:2}}

%%%%%%%%%%%%%%%%%%%%%%%%%%%%%
\section{Details of \cref{sec:3}}

\section{Details of \cref{sec:4}}
